# Supplementary material for: MIME: Human-Aware 3D Scene Generation
Source: arXiv:2212.04360 source file (2022-12-08)
Supplement: Supplementary file 1 [file 01_DATASET.tex]

\section{\datasetname}

\paragraph{How to put a contact human to interact with an object.}

\paragraph{More Examples.}
