# Supplementary material for: MIME: Human-Aware 3D Scene Generation
Source: arXiv:2212.04360 source file (2022-12-08)
Supplement: Supplementary file 2 [file 04_FAILURE_CASES.tex]

\section{Failure Cases.}
