# Supplementary material for: MIME: Human-Aware 3D Scene Generation
Source: arXiv:2212.04360 source file (2022-12-08)
Supplement: Supplementary file 3 [file 05_IPHONE_CASES.tex]

\section{Results on Different Motion Input}
